# Supplementary material for: Improving Question Answering with External Knowledge
Source: arXiv:1902.00993 source file (2019-10-01)
Supplement: Supplementary file 1 [file appendix.tex]

\section{Appendices}
\label{sec:appendix}

\begin{table*}[]
\centering
\small
\begin{tabular}{cccccc}
\toprule
\bf Base Model & \bf Input Sequence$^\ddagger$ & \bf Finetuning Datasets$^\dagger$ & \bf Weight& \bf Count \\
\midrule
GPT+SA+HL & $[o\$qd]$ & R+C & 1 & 1 \\
${\text{BERT}_\text{LARGE}}$ & $@d\#q\#o\#$ &  R+C & 1 & 7 \\
${\text{BERT}_\text{LARGE}}$ & $@q\#o\#d\#$ &  R+C & 1 & 4 \\
${\text{BERT}_\text{LARGE}}$ & $@d\#o\#q\#$ &  R+C & 1 & 4 \\
${\text{BERT}_\text{LARGE}}$ & $@d\#q\#o\#$ &  R+C+E+O & 3 & 2 \\
${\text{BERT}_\text{LARGE}}$ & $@o\#q\#d\#$ &  R+C+E+O & 3 & 2 \\
${\text{BERT}_\text{LARGE}}$ & $@d\#o\#q\#$ &  R+C+E+O & 3 & 3 \\
${\text{BERT}_\text{LARGE}}$ & $@q\#o\#d\#$ &  R+C+E+O & 3 & 3 \\
${\text{BERT}_\text{LARGE}}$ & $@q\#o\#d\#$ &  R+C+E & 3 & 1 \\
${\text{BERT}_\text{LARGE}}$ & $@q\#d\#o\#$ &  R+C+E+O & 3 & 1 \\
${\text{BERT}_\text{LARGE}}$ & $@o\#d\#q\#$ &  R+C+E+O & 3 & 1 \\
\bottomrule
\end{tabular}
\caption{Settings of ARC-Challenge Models. $^\dagger$: R (RACE), C (ARC-Challenge), E (ARC-Easy), O (OpenBookQA). $^\ddagger$: $[$ (start token in GPT), $\$$ (delimiter token in GPT), $]$ (end token in GPT), $@$ ($\texttt{[CLS]}$ token in BERT), $\#$ ($\texttt{[SEP]}$ token in BERT).} 
\label{tab:appendix:arc}
\end{table*}

\begin{table}[]
\centering
\small
\begin{tabular}{ccc}
\toprule
 \bf Input Sequence$^\ddagger$ & \bf Finetuning Datasets$^\dagger$ & \bf Count \\
\midrule
 $@d\#q\#o\#$ &  R+E &  2 \\ %
 $@q\#o\#d\#$ &  R+E &  2 \\ %
 $@d\#o\#q\#$ &  R+E &  1 \\  %
 $@o\#q\#d\#$ &  R+E &  4 \\ %
 $@q\#d\#o\#$ &  R+E &  2 \\ %
  $@d\#q\#o\#$ &  R+E+C+O &  1 \\ %
 $@d\#o\#q\#$ &  R+E+C+O &  2 \\ %
$@q\#o\#d\#$ &  R+E+C+O & 2 \\ %
$@q\#d\#o\#$ &  R+E+C+O &  1 \\ %
 $@o\#d\#q\#$ &  R+E+C+O &  1 \\ %
\bottomrule
\end{tabular}
\caption{Settings of ARC-Easy Models. $^\dagger$: R (RACE), C (ARC-Challenge), E (ARC-Easy), O (OpenBookQA). $^\ddagger$: $@$ ($\texttt{[CLS]}$ token in BERT), $\#$ ($\texttt{[SEP]}$ token in BERT).} 
\label{tab:appendix:arceasy}
\end{table}

\begin{table}[]
\centering
\small
\begin{tabular}{ccc}
\toprule
 \bf Input Sequence$^\ddagger$ & \bf Finetuning Datasets$^\dagger$  \\
\midrule
 $@d\#q\#o\#$ &  R+O  \\  %
 $@d\#o\#q\#$ &  R+O \\   %
 $@o\#q\#d\#$ &  R+O  \\  %
 $@q\#d\#o\#$ &  R+O \\  %
 $@d\#o\#q\#$ &  R+O*+E+C  \\ %
\bottomrule
\end{tabular}
\caption{Settings of OpenBookQA Models. $^\dagger$: R (RACE), C (ARC-Challenge), E (ARC-Easy), O (OpenBookQA), O* (OpenBookQA with 54.6\% instances dropped). $^\ddagger$: $@$ ($\texttt{[CLS]}$ token in BERT), $\#$ ($\texttt{[SEP]}$ token in BERT).} 
\label{tab:appendix:openbook}
\end{table}

\begin{table}[]
\centering
\small
\begin{tabular}{c}
\toprule
\bf Input Sequence \\
\midrule 
 $\underline{@d\#}q\#o\#$   \\
 $\underline{@q\#o\#}d\#$  \\
 $\underline{@d\#}o\#q\#$   \\
 $\underline{@o\#q\#}d\#$   \\
 $\underline{@q\#d\#}o\#$  \\
$\underline{@o\#d\#}q\#$   \\
\bottomrule
\end{tabular}
\caption{BERT Segmentation Embedding Settings for Different Input Sequences. We add segmentation embedding \texttt{A} to the \underline{underlined} part and \texttt{B} to the rest.} 
\label{tab:appendix:segembed}
\end{table}

\subsection{Engineering Details of the Strong Systems Used for Comparison}

When we were in the middle of paper preparation, to make a competitive comparison, we put semi-complex engineering effort into making strong systems for ARC-Challenge, ARC-Easy, and OpenBookQA. These systems employed the approach of concurrently fine-tuning on multiple target datasets (Section~\ref{sec:method:in-domain}), system ensembles based on a generalization of reading strategies~\cite{sun2018improving}, and different pre-trained language models~\cite{radfordimproving,bert2018}. We describe their details in this section.

\subsubsection{Approach Overview}

\begin{itemize}
    \item \textbf{Reference Documents} Given a question and an option, we employed the same approach as \citeauthor{sun2018improving} to retrieve relevant sentences from the corpus provided by each dataset and regard the concatenation of the retrieved sentences as the reference document (Section~\ref{sec:method:basic}). We did \textbf{not} leverage any further steps such as EDL (Section~\ref{sec:method:open-domain}) to enrich the reference document.

    \item \textbf{Pre-trained Language Models} We mainly employed BERT~\cite{bert2018} as the pre-trained language model. We used uncased $\text{BERT}_{\text{LARGE}}$ for all our BERT-based models. Besides, we also employed GPT~\cite{radfordimproving} for ARC-Challenge. 
    
    \item \textbf{Fine-Tuning Strategies} Following \citeauthor{sun2018improving}, all our models were first fine-tuned on the RACE dataset~\cite{lai2017race}. In our GPT-based model, we employed self-assessment (SA) and highlighting (HL) reading strategies~\cite{sun2018improving} and followed their input representation accordingly. In our BERT-based models, we generalized the back-and-forth reading strategy~\cite{sun2018improving} by training models with more diverse input sequence order and ensembling them simultaneously rather than only ensembling model pairs with reverse or almost reverse input sequence order. 
    \item \textbf{Utilization of In-Domain Data} We employed the approach of simultaneously fine-tuning on multiple target datasets described in Section~\ref{sec:method:in-domain} with the exception that we randomly dropped a portion of training instances in OpenBookQA when simultaneously fine-tuning on multiple target datasets for OpenBookQA.
\end{itemize}

\subsubsection{Settings for Each Tasks}
\begin{itemize}
    \item \textbf{ARC-Challenge}
    The system for ARC-Challenge was composed of 29 models (Table~\ref{tab:appendix:arc}). The final prediction for each question is the option with the largest weighted average logit, where we simply set weight 1 for all models that only use RACE and ARC-Challenge for fine-tuning and 3 for the other models. The BERT segmentation embedding settings for different input sequences are detailed in Table~\ref{tab:appendix:segembed}.

    \item \textbf{ARC-Easy} The system for ARC-Easy was composed of 18 models (Table~\ref{tab:appendix:arceasy}). Different from ARC-Challenge, we only employed ${\text{BERT}_\text{LARGE}}$, and all models have equal weights (\ie, the final prediction for each question is the option with the largest average logit).

    \item \textbf{OpenBookQA} The system for OpenBookQA was composed of 5 models (Table~\ref{tab:appendix:openbook}). Different from ARC, we employed only one model for each used input sequence. Moreover, we dropped 54.6\% OpenBookQA training instances when fine-tuning on multiple datasets. 

\end{itemize}

We trained our BERT-based models with the same settings as Section~\ref{sec:exp:settings} and our GPT-based model with the same settings as~\citeauthor{sun2018improving}.
